# Supplementary material for: DRAMA: Next-Gen Dynamic Orchestration for Resilient Multi-Agent Ecosystems in Flux
Source: arXiv:2508.04332 source file (2026-05-20)
Supplement: Supplementary file 1 [file X_suppl.tex]

\clearpage
\setcounter{page}{1}
\maketitlesupplementary
\appendix
\section{Details of the Experiments}
In this section, we explain some implementation details of our experiments.
\label{app:a}

\textbf{Dataset}
As noted in part experiment setup, we use the Communicative Watch-And-Help(C-WAH) benchmark. In fact, we are using the test set in this benchmark, which contains a total of 50 household tasks and includes five types of tasks, named \textit{Preparation}, \textit{Cleaning}, \textit{Cooking}, \textit{Groceries}, and \textit{Setting up} (Table \ref{tab:cwah-tasks}).

Since the original task set was designed for two agents, in order to adapt to the situation of more agents, the original 3-5 subgoals were modified to 8-15 subgoals, which to some extent increased the complexity of the tasks.
% 您可以使用 [h!] (尽量这里), [t] (页顶), 或 [b] (页底)
\begin{table}[h!] 
\centering
\caption{Task descriptions with relative objects}
\label{tab:cwah-tasks}

% 使用标准的 tabular 环境
% 将 X 列替换为 p{宽度} 列，以实现自动换行
\begin{tabular}{lp{0.6\linewidth}} 
\toprule
\textbf{Task Type} & \textbf{Relative Object} \\
\midrule
Preparation & 
cupcake, pudding, apple, juice, wine, coffeetable \\
\midrule
Cleaning &
plate, fork, dishwasher \\
\midrule
Cooking &
coffeepot, cupcake, pancake, poundcake, pudding, apple, juice, wine, dinnertable \\
\midrule
Groceries &
cupcake, pancake, poundcake, pudding, apple, juice, wine, fridge \\
\midrule
Setting up &
plate, fork, dinnertable \\
\bottomrule
\end{tabular}
\end{table}

\textbf{Baseline}
Due to task set adaptation reasons, all baseline methods are based on CoELA.
\begin{itemize}
    \item \textbf{CoELA}: Since CoELA itself is a framework designed for two agents, to support a greater number of agents, we use a modified version by Guo et al.
    \item \textbf{MCTS}: Use the original adapted MCTS in CoELA.
    \item \textbf{AgentVerse-Satic}: We designed a task allocator to assign roles and responsibilities to different agents.
    \item \textbf{AgentVerse-Dynamic}: Considering that there is an evaluator in AgentVerse that assesses the organizational structure after the task is completed, in static, since each task is independent, the evaluation would be meaningless. Therefore, we designed a more dynamic version and created an evaluator to evaluate the organizational structure when the sub-goals are completed.
    \item \textbf{ProAgent}: Transplant the intention prediction and belief revision involved in ProAgent.
\end{itemize}

\textbf{Dropout Processing}
In DRAMA, we have designed a set of processes, including having the agent dropout, drop detection and drop handling. In terms of handling lost contact, we processed the relevant information of the disconnected agent. In other methods, the failure to process this information would lead to the failure of the task. In the experiment, we added this processing flow to all the compared methods.

\section{Detailed experimental data}
To demonstrate the robustness and foundational effectiveness of our approach, this section presents results from a preliminary study conducted on the original C--WAH benchmark. This dataset represents a scenario with lower task complexity (i.e., fewer objects per task) compared to the extended environment in our main analysis.

The version of our method tested here, along with the baselines, utilizes foundational metrics: Average Steps (AS) for temporal efficiency and Total Steps (TS) for resource expenditure. While our main paper introduces a more advanced methodology and more fine-grained metrics (CR, TP) to analyze complex interactions, the results from this initial investigation (Table \ref{tab:cwah-metrics-origin}) were crucial. They established the core performance advantage of our agent coordination strategy, justifying the further development that led to the final version of DRAMA presented in the main paper. All trials were re-conducted in the event of a simulator-induced failure.

\definecolor{myblue}{RGB}{255, 200, 170}
\begin{table*}[t!]
\centering

\setlength{\tabcolsep}{6pt} % Adjusted column separation for better fit
\caption{A detailed comparison of all methods on the original C-WAH benchmark, featuring a reduced number of objects per task. Results are shown for both static scenarios (with 2, 3, and 4 agents) and dynamic scenarios involving agent dropout and addition.}
\label{tab:cwah-metrics-origin}
\begin{tabular}{ll|ccc|cc}
\toprule
& & \multicolumn{3}{c|}{\textbf{Static Scenarios}} & \multicolumn{2}{c}{\textbf{Dynamic Scenarios}} \\
\cmidrule(lr){3-5} \cmidrule(lr){6-7}
\textbf{Method} & \textbf{Metric} & \textbf{2 Agents} & \textbf{3 Agents} & \textbf{4 Agents} & \textbf{3 $\rightarrow$ 2} & \textbf{3 $\rightarrow$ 4} \\

\rowcolor{gray!20}
\multicolumn{7}{c}{\textit{Comparison Methods}} \\

\multirow{2}{*}{CoELA} & AS(Steps) & 70.32 & 52 & 49.58 & 60.58 & 54.47 \\
& TS(Steps) & 125.36 & 119 & 133.14 & 99.66 & 121.55 \\
\midrule
\multirow{2}{*}{MCTS} & AS(Steps) & 87.4 & 68 & 60.67 & 81.34 & 73.78 \\
& TS(Steps) & 140.08 & 135.22 & 132.28 & 135.89 & 172.60 \\
\midrule
\multirow{2}{*}{ProAgent} & AS(Steps) & 66.65 & 53.67 & 49.04 & 63.16 & 53.83 \\
& TS(Steps) & 109.78 & 114.73 & 123.52 & 104.80 & 121.54 \\
\midrule
\multirow{2}{*}{AV-Static} & AS(Steps) & 68.12 & 52.96 & 51.6 & 65.04 & 53.05 \\
& TS(Steps) & 113.22 & 110.38 & 131.82 & 107.82 & 125.30 \\
\midrule
\multirow{2}{*}{AV-Dynamic} & AS(Steps) & 68.54 & 57.48 & 51.5 & 67.90 & 61.91 \\
& TS(Steps) & 111.78 & 121.22 & 126.76 & 126.48 & 142.95 \\
\midrule
\rowcolor{gray!20}
\multicolumn{7}{c}{\textit{Our Method}} \\
\multirow{2}{*}{\textbf{DRAMA}} & \textbf{AS(Steps)} & \textbf{67.8} & \textbf{49.4} & \textbf{46.34} & \textbf{58.74} & \textbf{51.26} \\
& \textbf{TS(Steps)} & \textbf{110.38} & \textbf{98.6} & \textbf{102.2} & \textbf{99.96} & \textbf{116} \\
\bottomrule
\end{tabular}
\end{table*}

In the part of stableness of DRAMA, we choose the two tasks in the dataset. We ran in two different scenarios: dropout(5$\rightarrow$4) and addition (3$\rightarrow$5), each independently running 50 times to count AS (Average Steps), CR (Conflict Rate) and TP (Throughput). The detailed data is as follows (Table \ref{tab:cwah-stableness-detailed})

To validate the distinct contributions of our key architectural innovations, we conduct two critical ablation studies. We investigate the impact of: (1) removing the Collective Intelligence Layer, forcing agents to rely on blind search without semantic priors, and (2) disabling the Trust Chain mechanism, thus removing the system's explicit fault tolerance capability. All experiments are conducted on our most challenging dynamic scenarios, and the results are summarized in Table~\ref{tab:ablation}.

\begin{table*}[t!]
\centering

\setlength{\tabcolsep}{5pt} % Reduced padding to fit more columns
\caption{Detailed statistical comparison of DRAMA against baselines under dynamic scenarios for Average Steps (AS), Conflict Rate (CR), and Throughput (TP).}
\label{tab:cwah-stableness-detailed}
\begin{tabular}{l|cccc|cccc|cccc}
\toprule
& \multicolumn{4}{c|}{\textbf{AS}} & \multicolumn{4}{c|}{\textbf{CR}} & \multicolumn{4}{c}{\textbf{TP}} \\
\cmidrule(lr){2-5} \cmidrule(lr){6-9} \cmidrule(lr){10-13}
\textbf{Method} & \textbf{Mean} & \textbf{Var} & \textbf{Min} & \textbf{Max} & \textbf{Mean} & \textbf{Var} & \textbf{Min} & \textbf{Max} & \textbf{Mean} & \textbf{Var} & \textbf{Min} & \textbf{Max} \\
\midrule
\rowcolor{gray!20}
\multicolumn{13}{c}{\textbf{Dynamic: 5 Agents to 3 Agents}} \\
CoELA       & 63.2   & 73.16  & 46 & 85   & 0.0718 & 0.0013 & 0.0152 & 0.1786 & 0.2417 & 0.0011 & 0.1765 & 0.3261 \\
ProAgent    & 63.68  & 114.86 & 42 & 90   & 0.1245 & 0.0021 & 0.0435 & 0.25   & 0.2431 & 0.0021 & 0.1667 & 0.3571 \\
AV-Static   & 60.82  & 94.63  & 43 & 87   & 0.0505 & 0.0017 & 0      & 0.1724 & 0.2529 & 0.0016 & 0.1724 & 0.3488 \\
AV-Dynamic  & 63.2   & 115.84 & 45 & 91   & 0.05   & 0.0014 & 0      & 0.1852 & 0.2439 & 0.0015 & 0.1648 & 0.3333 \\
\textbf{DRAMA}& \textbf{56.44} & \textbf{67.45} & \textbf{39} & \textbf{76} & \textbf{0.0372} & \textbf{0.0008} & \textbf{0} & \textbf{0.0933} & \textbf{0.2715} & \textbf{0.0016} & \textbf{0.1974} & \textbf{0.3846} \\
\midrule
\rowcolor{gray!20}
\multicolumn{13}{c}{\textbf{Dynamic: 3 Agents to 5 Agents}} \\
CoELA       & 56.5   & 60.33  & 37 & 72   & 0.104  & 0.0025 & 0.0164 & 0.2128 & 0.2709 & 0.0016 & 0.2083 & 0.4054 \\
ProAgent    & 54.56  & 35.41  & 41 & 70   & 0.1088 & 0.0024 & 0      & 0.193  & 0.2783 & 0.001  & 0.2143 & 0.3659 \\
AV-Static   & 54.86  & 48.64  & 45 & 87   & 0.0537 & 0.0019 & 0      & 0.2041 & 0.2779 & 0.0013 & 0.2113 & 0.3571 \\
AV-Dynamic  & 60.44  & 78.17  & 42 & 71   & 0.0469 & 0.0013 & 0      & 0.1765 & 0.2535 & 0.0014 & 0.1724 & 0.3333 \\
\textbf{DRAMA}& \textbf{52.1}  & \textbf{40.41} & \textbf{39} & \textbf{65} & \textbf{0.0457} & \textbf{0.001}  & \textbf{0} & \textbf{0.1628} & \textbf{0.2923} & \textbf{0.0013} & \textbf{0.2308} & \textbf{0.3846} \\
\bottomrule
\end{tabular}
\end{table*}

\begin{table*}[!ht]
\centering
\caption{\textbf{Ablation study on the core components of our framework.} 
Performance of the full model versus variants lacking the Collective Intelligence Layer and the Trust Chain mechanism across all test scenarios.}
\label{tab:ablation}
\resizebox{\textwidth}{!}{%
\begin{tabular}{lcccccccccc}
\toprule
& & \multicolumn{3}{c}{\textbf{Static}} & \multicolumn{2}{c}{\textbf{Dropout}} & \multicolumn{2}{c}{\textbf{Addition}} & \multicolumn{1}{c}{\textbf{Recovery}}& \multicolumn{1}{c}{\textbf{Replacement}} \\
\cmidrule(lr){3-5} \cmidrule(lr){6-7} \cmidrule(lr){8-9} \cmidrule(lr){10-10}  \cmidrule(lr){11-11}
\textbf{Method} & \textbf{Matrix} 
& \textbf{3} & \textbf{4} & \textbf{5}
& \textbf{4$\rightarrow$3} & \textbf{5$\rightarrow$4$\rightarrow$3}
& \textbf{4$\rightarrow$5} & \textbf{3$\rightarrow$4$\rightarrow$5}
& \textbf{4$\rightarrow$3$\rightarrow$4} & \textbf{4$\rightarrow$3$\rightarrow$4$^{\prime}$}\\

\midrule

% ================= Full Model =================
\multirow{3}{*}{Full Model (Ours)}
& AS & 59.977 & 50.242 & 46.697 & 57.205 & 52.796 & 48.213 & 53.367 & 55.609 & 55.429 \\
& CR & 0.027 & 0.062 & 0.083 & 0.026 & 0.076 & 0.068 & 0.057 & 0.044 & 0.061 \\
& TP & 0.189 & 0.217 & 0.252 & 0.2 & 0.216 & 0.235 & 0.211 & 0.204 & 0.205 \\
\midrule

% ================= w/o Collective Intelligence Layer =================
\multirow{3}{*}{w/o Collective Intelligence Layer}
& AS & 65.432 & 56.674 & 48.043 & 61.021 & 57.659 & 53.918 & 54.918 & 57.767 & 60.78 \\
& CR & 0.037 & 0.054 & 0.119 & 0.029 & 0.079 & 0.073 & 0.064 & 0.062 & 0.059 \\
& TP & 0.171 & 0.205 & 0.242 & 0.188 & 0.211 & 0.211 & 0.208 & 0.198 & 0.186 \\
\midrule

% ================= w/o Trust Chain mechanism =================
\multirow{3}{*}{w/o Trust Chain mechanism}
& AS & 61.644 & 53.367 & 45.14 & 60.851 & 54.381 & 49.837 & 55.52 & 57.083 & 58.804 \\
& CR & 0.022 & 0.046 & 0.104 & 0.044 & 0.079 & 0.072 & 0.061 & 0.049 & 0.056 \\
& TP & 0.182 & 0.214 & 0.263 & 0.189 & 0.213 & 0.22 & 0.207 & 0.197 & 0.194 \\
\bottomrule
\end{tabular}%
}
\end{table*}

\section{Experiment Environment}
This environment is running on Unity Simulator version linux\_exec.v2.3.0, equipped with an NVIDIA 4090 GPU and a 32 vCPU Intel(R) Xeon(R) Platinum 8352V CPU at 2.10GHz. It supports CUDA 11.8 and uses Python 3.8.0.

\section{Implementation Details of the Probabilistic Belief Network}
\label{app:belief_network}

To enable agents to reason about object locations under uncertainty, our framework includes a probabilistic belief network for each object, parameterized by a lightweight Multi-Layer Perceptron (MLP). This network's primary role is not to memorize locations, but to learn a \textbf{generalizable belief update function}. It maintains a categorical distribution over potential rooms for each object, updating its belief based on sparse evidence from \texttt{[grab]} actions. This section details its architecture, its efficient training regime, and its operational logic.

\subsection{Problem Formulation and Architecture}
The core task is to maintain and update a belief distribution $\mathbf{p}(o) \in \Delta^{n-1}$ for each object $o$ over $n$ possible rooms, where $\Delta^{n-1}$ is the $(n-1)$-simplex.

\begin{itemize}
    \item \textbf{Network Input:} The MLP takes a $2n$-dimensional feature vector as input, which is a concatenation of the prior belief and the current observation: $\mathbf{x} = [\mathbf{p}_{t-1}, \mathbf{o}_t]$.
    \begin{itemize}
        \item $\mathbf{p}_{t-1} \in \mathbb{R}^n$: The belief distribution over rooms from the previous step.
        \item $\mathbf{o}_t \in \mathbb{R}^n$: A one-hot encoding of the room where a \texttt{[grab]} action occurred.
    \end{itemize}
    \item \textbf{MLP Architecture:} The network is a simple yet effective MLP with one hidden layer: 
    $$ \text{Linear}(2n \rightarrow 64) \rightarrow \text{ReLU} \rightarrow \text{Linear}(64 \rightarrow n) $$
    The output is a vector of $n$ logits. A Softmax function is applied during inference to produce the final probability distribution. A fixed, consistent ordering of rooms is used to ensure vector alignment.
\end{itemize}

\subsection{Few-Shot Online Training and Belief Update}
A key feature of our design is its exceptional data efficiency. The network is trained online using a minimal dataset to learn a robust belief update policy.

\begin{itemize}
    \item \textbf{Training Data:} The MLP is pre-trained on a small, representative dataset consisting of \textbf{only one trajectory from each of the five unique task types}. This ``five-shot'' training approach is designed to teach the model a general rule for how to update a belief given an observation, rather than overfitting to specific object locations.
    \item \textbf{Training Trigger:} After pre-training, the model continues to learn online. A single gradient step is performed each time an agent executes a \texttt{[grab]} action for a tracked object.
    \item \textbf{Objective:} The network is trained using a standard Cross-Entropy loss on the output logits, with the one-hot vector of the observed room $\mathbf{o}_t$ as the target label.
    \item \textbf{Inference and Update Logic:} Upon a new observation $\mathbf{o}_t$, the new belief $\mathbf{p}_t$ is computed via a stable blending process:
    \begin{enumerate}
        \item \textbf{Prediction:} $\mathbf{p}_{\text{net}} = \text{Softmax}(\text{MLP}([\mathbf{p}_{t-1}, \mathbf{o}_t]))$.
        \item \textbf{Blending:} $\mathbf{p}_{\text{blend}} = (1 - \eta) \cdot \mathbf{p}_{t-1} + \eta \cdot \mathbf{p}_{\text{net}}$, where $\eta=0.9$.
        \item \textbf{Normalization \& Write-back:} The blended vector is L1-normalized and persisted.
    \end{enumerate}
\end{itemize}

\subsection{Initialization, Persistence, and Hyperparameters}
The system is designed for continuous learning and persistence across tasks.

\begin{itemize}
    \item \textbf{Initialization:} The system loads the pre-trained MLP weights and a JSON file containing the last known belief distributions for all objects (priors). If a prior for an object does not exist, a uniform distribution is used.
    \item \textbf{Persistence:} At the end of each task, the updated MLP weights (saved as \texttt{mlp.pt}) and the latest object belief maps (saved as \texttt{global\_prob\_maps.json}) are written to disk.
    \item \textbf{Key Hyperparameters:} The system is configured with a hidden layer width of 64, a learning rate of $1 \times 10^{-3}$ for the Adam optimizer, and a blend factor of $\eta=0.9$.
\end{itemize}

% Optional: You can keep or remove the "Notes on Implementation" section based on space.

\subsection{Notes on Implementation}
The implementation is highly efficient, with the belief update being an $O(n)$ operation and the MLP forward/backward pass being computationally trivial on a CPU. The primary limitation is a potential cold-start problem, though the pre-training on five tasks and the blending mechanism help mitigate this.

\section{Prompts Templates}
We list the used prompts at Table \ref{tab:actor-prompt}.

\begin{table*}[ht]
\centering
\caption{Prompt of Actor.}
\label{tab:actor-prompt}

% Add a framebox around a minipage to create a bordered box
\fbox{
    \begin{minipage}{0.95\linewidth} % Adjust width as needed
    \ttfamily\small % Apply the desired font style and size

    % Manually add the title
    \textbf{Actor Prompts}
    \vspace{1em} % Add some space after the title

    % The original prompt text goes here
    "I'm \$AGENT\_NAME\$. I'm in a hurry to finish the housework with my friends \$TEAMMATE\_NAME\$ together. Given our shared goal, dialogue history, and my progress and previous actions, please help me choose the best available action to achieve the goal as soon as possible.
    
    Hard requirement:
    - The ""action"" you output MUST be exactly one of the lines listed under ""Available actions"" below. Copy it verbatim (including brackets, object ids, and punctuation). Do NOT invent actions. If no listed action is appropriate, use ""None"".

    Constraints and policy:
    
    - I can hold up to 2 objects.
    
    - Priority (strict):
    
      1) If a SubGoal object is visible and reachable, Take/Grab it.
      
      2) Else if any Goal object is visible and reachable, Take/Grab it.
      
      3) Else Navigate/Explore to the room with the highest SubGoal prior.
      
    - If target is inside a container, Open then Take.

    - If multiple targets are reachable, pick up up to 2.
    
    - If there are other agents in the same room with you, Take\\Grab the subgoal object first to avoid conflict with other agents.
    
    - Do NOT choose an action that targets the same object id or container id as any teammate in Previous actions (most recent step). Pick a different target/action instead.
    
    - If my agent number is larger than a teammate in the same room (e.g., Agent\_2 when Agent\_1 is present), assume earlier-index agents may choose the same target; proactively pick a different object/container or a different room to avoid taking the same action.
    
    - Tie-break: fewer steps; prefer immediate Take/Grab.

    Organization instructions: \$ORGANIZATION\_INSTRUCTIONS\$
    
    Goal: \$GOAL\$
    
    SubGoal: \$SUBGOAL\$
    
    Progress: \$PROGRESS\$
    
    Previous actions: \$ACTION\_HISTORY\$
    
    Available actions: \$AVAILABLE\_ACTIONS\$
    
    Response format:
    
    \{""thoughts"" : ""thoughts content"", 
    
    ""action"" : ""choose one action from the available actions above or None""\}
    
    Validation:
    
    - The ""action"" must be identical to one of the strings under ""Available actions"" (or ""None"" if nothing applies). Do not output any other string."
    \end{minipage}
}
\end{table*}

\section{Case Study}
\begin{figure*}
    \centering
    \includegraphics[width=1\linewidth]{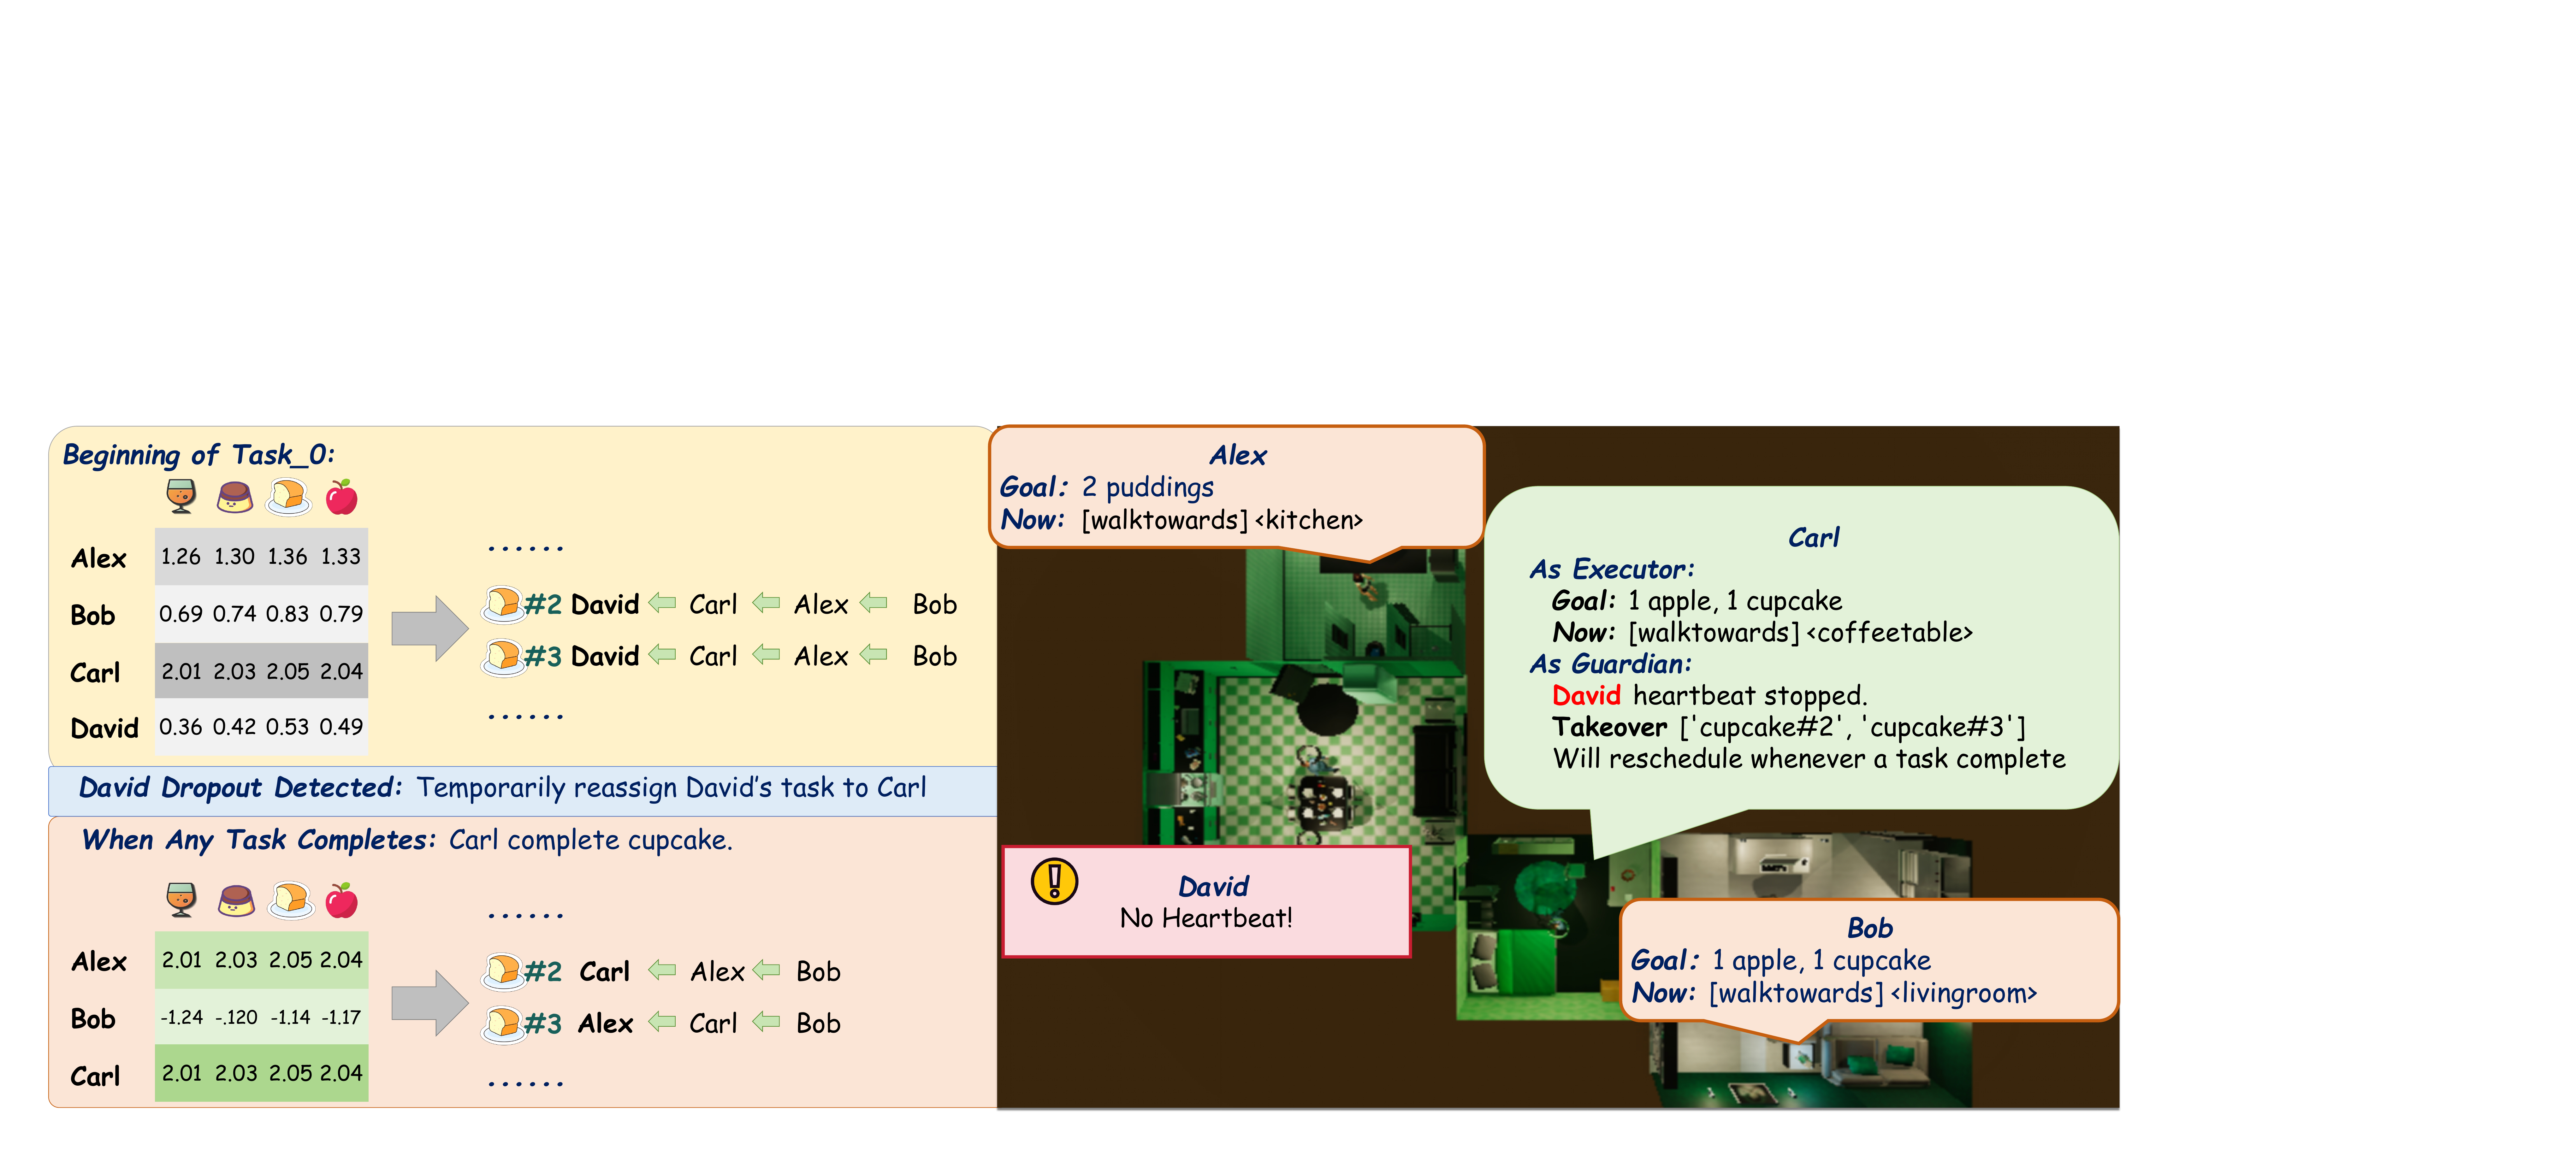}
    % \caption{A case study example of DRAMA occurring when Bob disconnects.}
    \caption{An example scenario demonstrating the dynamic adaptation of DRAMA after Bob disconnects.}
    \label{fig:case}
\end{figure*}
% As illustrated in Fig.~\ref{fig:case}, the system demonstrates robust adaptation to agent failure. When the monitor detects that Bob has become unresponsive in the living room, it flags the issue and triggers the control plane to reassign Bob’s tasks. The planner, observing that only Alice and Carter remain available—neither ideally positioned for Bob’s subtasks—randomly assigns these tasks to Carter. This reassignment is validated by the critic and enacted by the scheduler, ensuring no interruption in task execution.

As illustrated in Figure~\ref{fig:case}, the system demonstrates strong resilience to agent dropout events. 
During \textit{Task\_0}, all agents initially operate in coordinated fashion, with task affinities computed across Alex, Bob, Carl, and David. 
When the guardian mechanism detects that \textit{David} has lost connection in the living room (\textit{heartbeat stopped}), his primary guardian, \textit{Carl}, is promptly notified. 
Through the \textit{takeover module}, Carl temporarily assumes David’s remaining responsibilities—including the delivery of \texttt{cupcake\#2} and \texttt{cupcake\#3}—to prevent task interruption. 
This reassignment is transparently recorded within the guardian chain, preserving operational continuity and accountability at the team level.

When any worker agent completes a task, a rescheduling procedure is automatically triggered. 
In this episode, Carl completes a cupcake delivery, prompting the control plane to recompute the affinity matrix based on the updated workload and spatial configuration. 
Consequently, the scheduler redistributes the remaining subtasks and reconstructs the guardian chains to represent the revised agent–task dependencies. 
Meanwhile, Alex continues moving toward the kitchen to collect puddings, and Bob proceeds toward the living room to execute his assigned delivery. 
This dynamic coordination among the control, executor, and guardian pathways enables the team to adapt effectively to unexpected failures, maintaining stable progress toward the shared objective even under partial agent loss.

\section{Limitations}
Experiments are conducted in a simulated embodied environment, which may not fully capture the perception noise and actuator uncertainty of real-world systems. Extending DRAMA to physical multi-robot settings or mixed-reality platforms would validate its practicality under real-world constraints.
